# Supplementary material for: StreamSide: A Fully-Customizable Open-Source Toolkit for Efficient Annotation of Meaning Representations
Source: arXiv:2109.09853 source file (2021-09-20)
Supplement: Supplementary file 1 [file appendix.tex]

\section{Appendix}
\label{sec:appendix}
